# Supplementary material for: SPIN: Spacecraft Imagery for Navigation
Source: arXiv:2406.07500 source file (2024-12-05)
Supplement: Supplementary file 1 [file X_suppl.tex]

\clearpage
\setcounter{page}{1}
\maketitlesupplementary

\section{SPacecraft Imagery for Navigation}

As supplementary material for the SPacecraft Imagery for Navigation (SPIN) tool, we provide a functional demonstration of our simulation tool, a video summarising the tool's capabilities, and some additional examples of images generated with our simulator, and additional images comparing the model trained on our SPIN-generated dataset and the model trained on SPEED+.

\subsection{Demo Executable and Video}

Our paper introduces a simulation tool designed for dataset generation. As part of our contribution, we are providing a \textbf{demo} downloadable executable version for Windows, which offers a demonstration of the tool's capabilities with limited functionalities. The demo executable weighs about 600MB  and can be downloaded from: \href{https://github.com/CVPR2024ID5566/SPIN/releases/tag/Demo}{https://github.com/CVPR2024ID5566/SPIN/releases/tag/Demo}

We provide a screenshot of the demo SPIN executable in Figure~\ref{fig:spin-simulator}. Should our work be accepted, the complete tool and its code will be shared through GitHub and a dedicated webpage. Accompanying the demo, we offer a file with visual instructions for using the SPIN demo. Furthermore, we include a demonstration video that displays images created using various features of SPIN, illustrating the tool's capabilities.

\begin{figure}[h]
    \centering
    \includegraphics[width=\columnwidth]{fig_supp/simulator.png}
    \caption{Example screenshot from our SPIN Simulation tool. Please note this is a demo version with reduced functionalities.}
    \label{fig:spin-simulator}
\end{figure}

\subsection{Visual examples}

In this section, we provide additional rendering examples with our too. First, in Figure~\ref{fig:enhancement}, we provide more examples of the differences between images generated using a configuration aligned with the SPEED+ synthetic subset, and the same images after applying our enhancement settings. Next, in Figure~\ref{fig:additional-renderings} we display more examples of images that can be generated using our simulator, with different settings to the ones used for the SPEED+ like images.

\begin{figure*}[b]
    \centering
    \includegraphics[width=\textwidth]{fig_supp/enhacement.jpg}
    \caption{Image comparison between a baseline configured like the synthetic split from the SPEED+ dataset, and the same images after applying Environment, Camera, and Material settings.}
    \label{fig:enhancement}
\end{figure*}

\begin{figure}[h]
    \centering
    \includegraphics[width=.9\columnwidth]{fig_supp/fig2_v.png}
    \caption{Some examples of different renderings generated with our tool. Top right image depicts the keypoint visualization tool, whereas the rest of the images present different combinations of background, illumination, and color corrections.}
    \label{fig:additional-renderings}
\end{figure}

\section{Spacecraft Pose Estimation}

In this section, we provide further details on the pose estimation pipeline.

\subsection{Training Hyperparameters}
In Table~\ref{table:hyperparameters} we put the different hyperparameters used while training the different models. No parameters were modified between different models.

\begin{table}[h]
\centering

\begin{tabular}{|l|l|l|}
\hline
\textbf{Parameter} & \textbf{Value}  & \textbf{Description}\\ \hline
target\_size & [512, 512] & \parbox{4cm}{\vspace{2pt}Size of the input images.\vspace{2pt}}\\ \hline
std & 7 & \parbox{4cm}{\vspace{2pt}Standard deviation for the Gaussians for keypoint heatmaps in pixel units.\vspace{2pt}} \\ \hline
resnet\_size & 50 & \parbox{4cm}{\vspace{2pt} Size of the ResNet Backbone used. \vspace{2pt}} \\ \hline
mean\_img & 41.1280 & \parbox{4cm}{\vspace{2pt} Normalization parameter.\vspace{2pt}}\\ \hline
std\_img & 36.9064  & \parbox{4cm}{\vspace{2pt} Normalization parameter.\vspace{2pt}}\\ \hline
lr & 2.5e-4  & \parbox{4cm}{\vspace{2pt}Learning rate value.\vspace{2pt}}\\ \hline
batch\_size & 6 & \parbox{4cm}{\vspace{2pt}Batch size used in training. \vspace{2pt}}\\ \hline
epochs & 60 & \parbox{4cm}{\vspace{2pt}Amount of epochs the models were trained for.\vspace{2pt}}\\ \hline

\end{tabular}
\caption{Training hyperparameters}
\label{table:hyperparameters}
\end{table}

\subsection{Visual Examples}

In this section, we present a visual comparison of pose estimation results obtained from training with the original SPEED+ synthetic dataset and then on a replica created using the proposed SPIN tool with the image enhancements activated. In particular, we show the pose estimation results for visually challenging scenes in Figure~\ref{fig:sup-difficult-examples}, and for less complex visual scenes in Figure~\ref{fig:sup-easy-examples}. We can observe how the model trained over the images generated by SPIN reaches improved performance compared to the model trained on SPEED+ in situations more closely related to real-world situations, such as high contrast areas, poor lighting, or close-up views of the spacecraft. Differently, for simpler scenes where the spacecraft is well lit, or the whole shape can be recognized, the pose estimation performance of both models is similar.

%In addition, we provide an analysis of the top 1000 errors achieved by the model trained on the original SPEED+ synthetic dataset and the model trained on the SPIN replica in Table~\ref{tab:spin-vs-speed-1000} we summarise four figures that represent the orientation errors $S_q$ against the translation errors $S_v$. We can observe that the errors achieved with the SPEED+ training synthetic set are more concentrated in the higher areas, whereas the errors of SPIN are more homogeneous.

\begin{figure}
    \centering
    \includegraphics[width=.9\columnwidth]{fig_supp/difficult-examples.jpg}
    \caption{Examples of the estimated pose, over the Lightbox and Sunlamp subsets over visually challenging examples. The pose estimation results are represented as a wireframe model overlaid over the spacecraft. The solid blue represents the results trained over SPIN generated images, and dashed yellow trained SPEED+ images. }
    \label{fig:sup-difficult-examples}
\end{figure}

\begin{figure}
    \centering
    \includegraphics[width=.9\columnwidth]{fig_supp/easy-examples.jpg}
    \caption{Examples of the estimated pose, over the Lightbox and Sunlamp subsets over visually simpler examples. The pose estimation results are represented as a wireframe model overlaid over the spacecraft. The solid blue represents the results trained over SPIN generated images, and dashed yellow trained SPEED+ images. }
    \label{fig:sup-easy-examples}
\end{figure}

%\begin{table}
%\centering
%\begin{tabular}{c|c|c}
%  & SPIN (Ours) & SPEED+ \\
%  \midrule
%  \raisebox{\dimexpr 0.5\height+1.1cm\relax}[0pt][0pt]{\rotatebox[origin=c]{90}{Lightbox}} & \includegraphics[width=0.4\linewidth]{fig_supp/spin_lb.png} & \includegraphics[width=0.4\linewidth]{fig_supp/speed_lb.png} \\
%  \midrule
%  \raisebox{\dimexpr 0.5\height+1.1cm\relax}[0pt][0pt]{\rotatebox[origin=c]{90}{Sunlamp}} & \includegraphics[width=0.4\linewidth]{fig_supp/spin_sl.png} & \includegraphics[width=0.4\linewidth]{fig_supp/speed_sl.png} \\

%\end{tabular}
%\caption{Distribution of the top 1000 errors of the pose estimation algorithm trained over SPIN (left column) and SPEED+ (right column). The orientation errors $S_q$ are represented against the translation errors$S_v$. In addition, the overall pose error $S$ is represented with a colormap. The results are reported for the Lightbox and Sunlamp datasets.}
%\label{tab:spin-vs-speed-1000}
%\end{table}
